# Supplementary material for: Order-agnostic Identifier for Large Language Model-based Generative Recommendation
Source: arXiv:2502.10833 source file (2025-05-25)
Supplement: Supplementary file 1 [file 6_SI.tex]

\section{Appendix}\label{sec:appendix}
